# Supplementary material for: On the Societal Impact of Machine Learning
Source: arXiv:2510.23693 source file (2026-09-10)
Supplement: Supplementary file 1 [file paper3_SupplementaryMaterials.pdf]

# Supplementary Material for the paper: "Bias on Demand: A Modelling Framework That Generates Synthetic Data With Bias"

Joachim Baumann
University of Zurich
Zurich University of Applied Sciences
Zurich, Switzerland
baumann@ifi.uzh.ch

Alessandro Castelnovo*
Data Science & Artificial Intelligence,
Intesa Sanpaolo S.p.A.
Dept. of Informatics, Systems and Communication, Univ. Milano Bicocca
Milan, Italy
alessandro.castelnovo@intesasanpaolo.com

Riccardo Crupi*
Data Science & Artificial Intelligence,
Intesa Sanpaolo S.p.A.
Turin, Italy
riccardo.crupi@intesasanpaolo.com

Nicole Inverardi*
Data Science & Artificial Intelligence,
Intesa Sanpaolo S.p.A.
Milan, Italy
nicole.inverardi@intesasanpaolo.com

Daniele Regoli*
Data Science & Artificial Intelligence,
Intesa Sanpaolo S.p.A.
Milan, Italy
daniele.regoli@intesasanpaolo.com

**ACM Reference Format:**
Joachim Baumann, Alessandro Castelnovo, Riccardo Crupi, Nicole Inverardi, and Daniele Regoli. 2023. Bias on Demand: A Modelling Framework That Generates Synthetic Data With Bias . In *2023 ACM Conference on Fairness, Accountability, and Transparency (FAccT '23), June 12–15, 2023, Chicago, IL, USA.* ACM, New York, NY, USA, 9 pages. https://doi.org/10.1145/3593013.3594058

This Supplementary Material of the paper "Bias on Demand: A Modelling Framework That Generates Synthetic Data With Bias" is organised as follows: in Section S1 we describe in some details algorithmic and deployment bias, thus extending Section "Bias Landscape in ML" of the main paper, where we focused on biases involved in data generation. In Section S2 we provide additional details related to the section "Experiments" of the main paper, as well as results and visualisations for additional experiments.

## S1 OTHER TYPES OF BIAS

### S1.1 Bias From Algorithm to User

Biases going *from algorithm to user* impact the resulting predictor, which is then used to inform decisions [44].

**Algorithmic bias** may occur whenever the algorithmic outcomes affect the behaviour of users. i.e. the bias is generated purely by the algorithm using unbiased data. There are different specific aspects of the ML pipeline that can result in *algorithmic bias* [54]:

*The views and opinions expressed are those of the authors and do not necessarily reflect the views of Intesa Sanpaolo, its affiliates or its employees.

Permission to make digital or hard copies of part or all of this work for personal or classroom use is granted without fee provided that copies are not made or distributed for profit or commercial advantage and that copies bear this notice and the full citation on the first page. Copyrights for third-party components of this work must be honored. For all other uses, contact the owner/author(s).
*FAccT '23, June 12–15, 2023, Chicago, IL, USA*
© 2023 Copyright held by the owner/author(s).
ACM ISBN 979-8-4007-0192-4/23/06.
https://doi.org/10.1145/3593013.3594058

*Aggregation bias*[1] arises when just one ML model is used for everyone even though there are subgroups for which a different model would be better suited due to heterogeneity w.r.t. the mapping of the features to the labels, i.e. the probability of having a label given some features. *Learning bias* occurs when the algorithmic design choices (such as the specified learning objective function or regularisation techniques) are not equally suited for all subgroups. *Evaluation bias* bias occurs if the benchmark dataset or the metrics used to assess the performance do not appropriately capture the relevant target population for which the system is ultimately used. In line with [44], we combine *aggregation bias*, *learning bias*, and *evaluation bias* using the umbrella term *algorithmic bias*: what these three variations of *algorithmic bias* have in common is that they all exacerbate performance disparities on underrepresented groups. Thus, they are going *from algorithm to user* in that they affect the learned predictor in a way that it results in unintended harmful consequences despite using an unbiased dataset [44].

Figure S1a shows an illustrative representation of biases that can arise during the algorithmic development, i.e. downstream with respect to the dataset generation. In this paper, our main focus lies in the generation of a biased dataset. Nevertheless, one could easily simulate this type of bias as well, e.g. by translating the graph into the following equation:

$$\hat{Y} = \hat{f}(\widetilde{X}) - \beta^{\hat{Y}} A, \tag{S1}$$

where $\beta^{\hat{Y}}$ denotes the magnitude of *algorithmic bias*.

### S1.2 Bias From User to World

Biases going *from user to world* impact the way final decisions are made and may thereby end up causing harmful consequences.

[1]Notice that Mehrabi et al. [44] describe *aggregation bias* as a type of bias that goes *from data to algorithm*, whereas Suresh and Guttag [54] count it towards the biases arising during the model building stage as it represents a limitation on the learned predictor. Here, we follow Suresh and Guttag [54]'s interpretation.

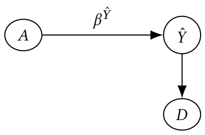


**(a) Algorithmic bias on $\hat{Y}$**

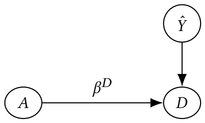


**(b) Deployment bias on $D$**

**Figure S1: Illustrative representation of biases involving the algorithm and its deployment – see also Equations** (S1) **and** (S2)**.**

**Deployment bias** arises if the process followed to take decisions based on the algorithm's prediction results in harmful downstream consequences. *Deployment bias* often occurs when predictions are used to inform human decision-makers, whereas the system has been created as if the decision would be taken fully automated based on the algorithmic predictions [54]. It is difficult to model all possible ways in which human decision-makers may act on the predictions, as this can be the result of complex processes in reality. Extending Mehrabi et al. [44]'s classification, *deployment bias* can be seen as a type of bias that is going *from user to world*, as it affects the way users of algorithmic decision-making systems derive (potentially consequential) decisions on individuals in the world.

Figure S1b shows an illustrative representation of biases that can arise during the algorithmic deployment, i.e. downstream with respect to the dataset generation. Similar to the *algorithmic bias* described above, one could easily simulate this type of bias as well, e.g. by translating the graph into the following equation:

$$D = r(\hat{Y}) - \beta^{D} A, \tag{S2}$$

where $\beta^{D}$ and represents the magnitude of *deployment bias*.

# S2 ADDENDUM ON EXPERIMENTS AND RESULTS

In this section, we provide additional experiments and results with respect to the main paper. First, we list the exact parameters used for all the experiments in Section S2.1. Then, in Section S2.2, we provide additional results for the two examples described in the section "Experiments" of the main paper. In Section S2.3, we provide results for other (combinations of) biases. Finally, in Section S2.4 we discuss an experiment where a non-linear implementation of (measurement) bias is introduced.

## S2.1 Parameters Used for the Experiments

For the experiments described in the section "Experiments" of the main paper we draw, for each scenario, $10^5$ observations generated with Equations (5)-(6). The $\beta$ parameters, i.e. those controlling bias presence and magnitude, are chosen according to the specific scenario, as described in "Experiments" of the main paper. The remaining parameters, i.e. those not directly involving bias, are instead fixed as by Table S1.

**Table S1: Fixed parameters for all experiments**

| $p_A$ | $k_R$ | $\theta_R$ | $K$ | $\alpha_{RQ}$ | $\alpha_R$ | $\alpha_Q$ | $\sigma_S$ | $\sigma_{P_S}$* | $\sigma_{P_R}$* |
|---|---|---|---|---|---|---|---|---|---|
| 0.5 | 2 | 3 | 3 | 0 | 1 | 2 | 2 | 2 | 2 |

* used only for the corresponding measurement bias scenario

The parameters $k_R$ and $\theta_R$ denote the shape and the scale, respectively, of the Gamma distribution used for the feature $R$. $K$ is the number of possible classes of the categorical variable $Q$. The parameter $p_A$ represents the probability of the Bernoulli distribution of variable $B_A$, indicating the proportion of individuals with $A = 1$. The standard deviations of the three Gaussian variables $S$, $P_S$, and $P_R$ are denoted by $\sigma_S$, $\sigma_{P_S}$, and $\sigma_{P_R}$, respectively. These parameters govern how likely is for each sampled instance to differ from the mean.

$\alpha_{RQ}$ denotes the strength of the relationship between $Q$ and $R$. The rationale is that of having a simple categorical distribution, but dependent on $R$ (and possibly $A$) with varying strength by tuning $\alpha_{RQ}$. Analogously $\alpha_R$ ($\alpha_Q$) governs the strength of the relation between $R$ ($Q$) and $Y$.

For all experiments, 2/3 of the $10^5$ observations are used to train the ML model and the remaining 1/3 are used as test set.

Table S2 lists a selection of (combinations of) different types of biases we chose to investigate using our synthetic bias generator along with the magnitudes (i.e. the values we specified for the corresponding bias parameter) we considered for each of them. For each scenario, all bias parameters not listed in Table S2 are fixed as 0 (as 'False' for omission bias).

## S2.2 Additional Visualisations for Experiments on Biased Features and Labels

Figure S2 shows the calibration plot for different magnitudes of measurement bias on the label $Y$. It shows that the predictor is always calibrated against the biased label $P_Y$ for group $A = 1$. However, with increasing bias of the label $Y$ (i.e. increasing values for $\beta_m^Y$), the predictor becomes less and less calibrated against the true label $Y$.

Figures S3 and S4 show the results for additional bias mitigation techniques (compared to the more concise Figures 4 and 5 described in the section "Discussion and Conclusion" of the main paper).

In Figure S5, we plot the correlation between the sensitive attribute $A$ and other variables, showing the impact of certain types of biases.

## S2.3 Additional Experiments

In this section, we provide the results for (combinations of) other types of biases.

As a reference point, we show the accuracy and fairness metrics for the dataset that does not contain any biases, i.e. all bias parameters are set to 0. The generative model is $Y = f(R, Q) + \epsilon$ and $R, Q \perp\!\!\!\perp A$. As can be seen in Figure S6, this results in an accuracy of 0.86 with acceptance rates of 0.43, TPR of 0.82, FPR of 0.11, PPV

**Table S2: Bias parameters used for the experiment**

| Bias type | Bias parameter | Values |
|---|---|---|
| no bias | - | - |
| measurement bias on $R$ | $\beta_m^R$ | 0, 0.1, 0.5, 1, 1.5, 2, 3, 4, 5, 6, 7, 8, 9 |
| measurement bias on $Y$ | $\beta_m^Y$ | 0, 0.1, 0.5, 1, 1.5, 2, 3, 4, 5, 6, 7, 8, 9 |
| historical bias on $R$ | $\beta_h^R$ | 0, 0.1, 0.5, 1, 1.5, 2, 3, 4, 5, 6, 7, 8, 9 |
| historical bias on $Y$ | $\beta_h^Y$ | 0, 0.1, 0.5, 1, 1.5, 2, 3, 4, 5, 6, 7, 8, 9 |
| historical bias on $Q$ | $\beta_h^Q$ | 0, 0.1, 0.5, 1, 1.5, 2, 3, 4, 5, 6, 7, 8, 9 |
| undersampling | $p_u \perp\!\!\!\perp R$ | 0.01, 0.008, 0.006, ..., 0.0002, 0.0001, 0.00009 |
| representation bias | $p_u \not\perp\!\!\!\perp R$ | 1, 0.8, 0.6, ..., 0.025, 0.01, 0.005, 0.001, 0.0005 |
| omission bias | - | True, False |
| historical bias and measurement bias on $R$ | $\beta_h^R, \beta_m^R$ | 0, 0.1, 0.5, 1, 1.5, 2, 3, 4, 5, 6, 7, 8, 9 |
| historical bias and measurement bias on $Y$ | $\beta_h^Y, \beta_m^Y$ | 0, 0.1, 0.5, 1, 1.5, 2, 3, 4, 5, 6, 7, 8, 9 |

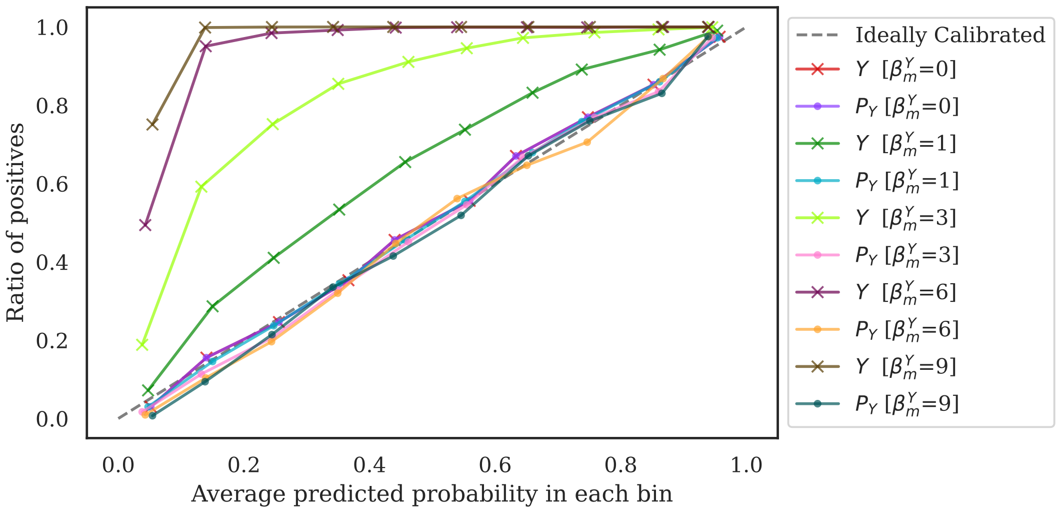


**Figure S2: Calibration plot for measurement bias on $Y$**

of 0.86, and FOR of 0.14 for both groups. Absent any bias, all group fairness parity criteria are satisfied.

Figure S7 shows the results for a dataset with different magnitudes of historical bias on $Q$. This case is very similar to the one presented in the section "Example 1: Biased Features in College Admissions" in the main paper. In both cases, there is historical bias on features. However, here we consider historical bias on $Q$ rather than on $R$. Since, in our implementation, the effect of $Q$ on $Y$ is smaller than the effect of $R$ on $Y$ (i.e. $\alpha_Q < \alpha_R$), less unfairness is produced in the case of historical bias on $Q$. Also, we can see in Figure S7 that unfairness (as measured with the different group fairness metrics described in Table 1 of the main paper), does not increase linearly with increasing historical bias on $Q$ (i.e. with increasing values for $\beta_h^Q$), but reaches a stable point with $\beta_h^Q \approx 4$. As in the case of historical bias on $R$ (see section "Example 1: Biased Features in College Admissions" of the main paper), Figure S7 shows that none of the bias mitigation techniques manages to fully get rid of all historical bias. Instead, they all improve fairness w.r.t. some group fairness metrics but at the same time worsen in for other group fairness metrics. If $DP$ is enforced to counteract the historical bias on the features, the accuracy only drops slightly in the case of historical bias on $Q$, in contrast to a considerable accuracy reduction in the case of historical bias on $R$.

Figure S8 shows an example in which the group $A = 1$ is undersampled in the dataset. As can be seen, apart from degenerate cases, random undersampling has no effect whatsoever on the fairness metrics and the overall performance. Thus, random undersampling per se is not enough to generate disparities among groups. Consequently, none of the bias mitigation techniques has any effect.

In contrast to random undersampling ($p_u \perp\!\!\!\perp R$), undersampling one group conditional on a relevant feature $R$ (i.e. $p_u \perp\!\!\!\perp R$) results in representation bias. As shown in Figure S9, representation bias

generates unfairness. In particular, it results in large *acceptance rate* and *TPR disparities* across groups $a \in A$. However, as is the case for random undersampling, once the sample of group $A = 1$ becomes very small (i.e. $p_u < 0.1$), the fairness and performance results become very unstable and are not meaningful anymore. Interestingly, in the case of representation bias, the selection rate of the group $A = 0$ stays roughly the same across all bias mitigation techniques and for any value of $p_u$ (apart from the negligible case of very low values). This happens since, in the implementation of representation bias in the synthetic data generator, we only change the representation of one of the two groups, i.e. we undersample the group $A = 1$. In particular, our implementation selects the individuals of the group $A = 1$ with lower values for $R$, which is why their acceptance rate decreases with higher values for $p_u$.

Let us now consider the case of omitting the feature $R$ so that the training set only contains $Q$ and $A$. This reduces the ML model's accuracy. As shown in Figure S10, it slightly increases the acceptance rate for both groups in this case. However, omitting a feature from the dataset generally does not generate any between-group disparities absent any other biases. If there is any other bias present in the dataset, omitting one of the features can very well have an effect on accuracy or fairness, for example, if the information included in the omitted variable could be used by the model to avoid those biases.

Next, we provide results for experiments using generated datasets that contain more than one type of bias at the same time. Figure S11 shows the results for a case with historical and measurement bias on $R$. This combines cases *a)* and *b)* from the college admissions example described in the section "Example 1: Biased Features in College Admissions" in the main paper. Figure S12 shows the results for a case with historical and measurement bias on $Y$. This combines cases *a)* and *b)* from the financial lending example described in the the section "Example 2: Biased Labels in Financial Lending" in the main paper.For both experiments, we choose the same magnitudes for both biases. I.e. the x-axis of Figures S11 and S12 corresponds to the magnitudes of historical bias and measurement bias: $\beta_h^j$ and $\beta_m^j$ for $j \in \{R, Y\}$.

As seen in both Figures, combining historical and measurement bias results in an accumulation of the effects observed when considering the two types of bias in isolation. However, different types of bias could, in theory, also render each other superfluous, e.g., with a lot of undersampling of one group, the biases present in this group in the data may become less prevalent. But, overall, the results for experiments with more than one type of bias in the data are more difficult to interpret. More research is needed to fully understand the interplay between many different types of bias present in a dataset at once.

## S2.4 Non-linear measurement bias on $Y$

In this section, we want to show how the results discussed in the section "Example 2: Biased Labels in Financial Lending" in the main paper change when the implementation of measurement bias on the target variable $Y$ is *non-linear*. Namely, we change Equation (6b) in the main paper (i.e., $P_S = S - \beta_m^Y A + N_{P_S}$) – where the dependence of $P_Y$ on $A$ is uniform across all instances – so that the skew in the proxy $P_Y$ with respect to $A$ is dependent on $R$. In particular, we 'penalise' (i.e. we flip the label from $Y = 1$ to $Y = 0$) individuals of the group $A = 1$ with $R$ lower than the median value $\widetilde{R}$, while we 'favour' (i.e. we flip the label from $Y = 0$ to $Y = 1$) individuals of the group $A = 1$ with $R$ above $\widetilde{R}$. We report here the full system of Equations (5)-(6) of the main paper with the specific implementation and values of parameters used for this experiment:

$$A = B_A, \quad B_A \sim \mathcal{B}er(0.5); \tag{S3a}$$

$$R = N_R, \quad N_R \sim Gamma(2,3); \tag{S3b}$$

$$Q = B_Q, \quad B_Q \sim \mathcal{B}in(3, 0.5); \tag{S3c}$$

$$S = R - Q + N_S, \quad N_S \sim \mathcal{N}(0, 2^2); \tag{S3d}$$

$$Y = \mathbf{1}_{\{S > \overline{P_S}\}}; \tag{S3e}$$

$$P_S = S - \beta_m^Y A \left(\mathbf{1}_{\{R < \widetilde{R}\}} - \mathbf{1}_{\{R \geq \widetilde{R}\}}\right) + N_{P_S}, \; N_{P_S} \sim \mathcal{N}(0, 2^2); \tag{S3f}$$

$$P_Y = \mathbf{1}_{\{P_S > \overline{P_S}\}}. \tag{S3g}$$

Suppose $A$ and $R$ denote individuals' gender and salary, respectively. In this case, the measurement bias on $Y$, as defined in Equation (S3f), represents a situation in which bank clerks are *less* lenient with loan repayment deadlines for women (denoted by $A = 1$) with a *low* salary while also being *more* lenient towards women with a *high* salary, compared to men (denoted by $A = 0$). In contrast, the example presented in the section "Example 2: Biased Labels in Financial Lending" in the main paper depicts a situation where bank clerks are less lenient towards women in general, regardless of their salary.

Figure S13 shows the values of group fairness metrics with increasing measurement bias $\beta_m^Y$. Notice that error-based metrics are computed with respect to the "true" target variable $Y$.

A model solely based on $R$ and $Q$ and blind to the sensitive attribute $A$ shows no dependence on $A$. This effect persists irrespective of the specific implementation of the measurement bias on $Y$. Since the "true" target variable $Y$ is independent of $A$ as well, i.e. the only dependence on the sensitive variable $A$ is in the measured proxy $P_Y$, FTU can mitigate the bias w.r.t. all fairness metrics, just as in the linear implementation of measurement bias on $Y$ (as discussed in the section "Example 2: Biased Labels in Financial Lending" in the main paper).

On the other hand, enforcing DP through post-processing the predicted scores yields a different result since those scores are produced with a prediction model that has access to the biased labels $P_Y$ and the sensitive attribute $A$ during training and prediction. The group-specific thresholds manage to achieve equal acceptance rates (i.e. a DP difference of zero) but without much effect on other metrics. This is indeed expected: as pointed out in the section "Example 2: Biased Labels in Financial Lending" in the main paper,the fact that enforcing DP is able to fully mitigate all group fairness disparities is an artefact of the implementation of measurement bias as a linear homogeneous shift in the proxy $P_Y$ (Equation (6b) in the main paper), but it is not a general property of measurement bias on $Y$. Furthermore, irrespective of the specific implementation of the measurement bias on $Y$, enforcing any other fairness constraint fails, as they all depend on the biased proxy $P_Y$.

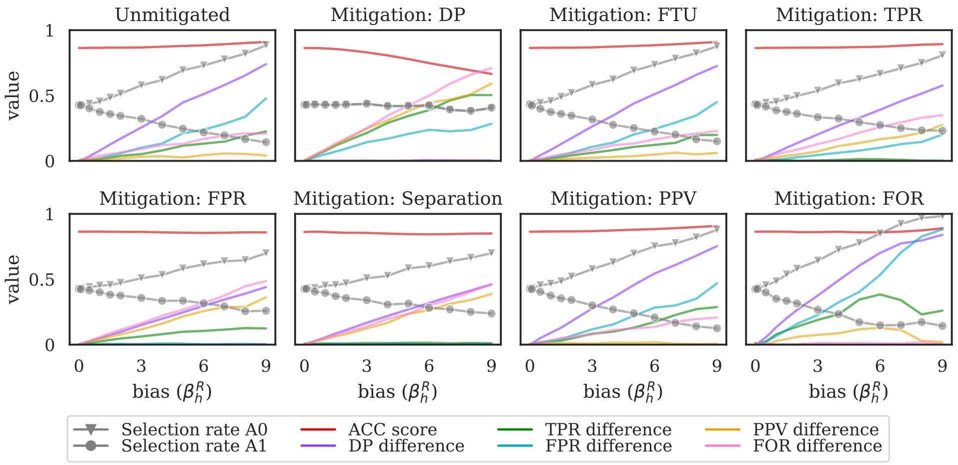


**(a) Historical bias on $R$**

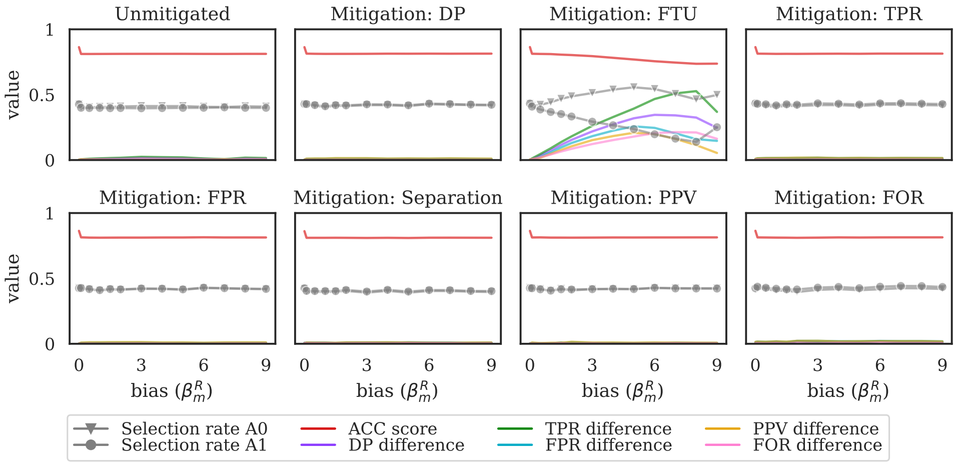


**(b) Measurement bias on $R$**

**Figure S3: Accuracy and fairness metrics for biased features $R$ in the college admission example (see section "Example 1: Biased Features in College Admissions" in the main paper.)**

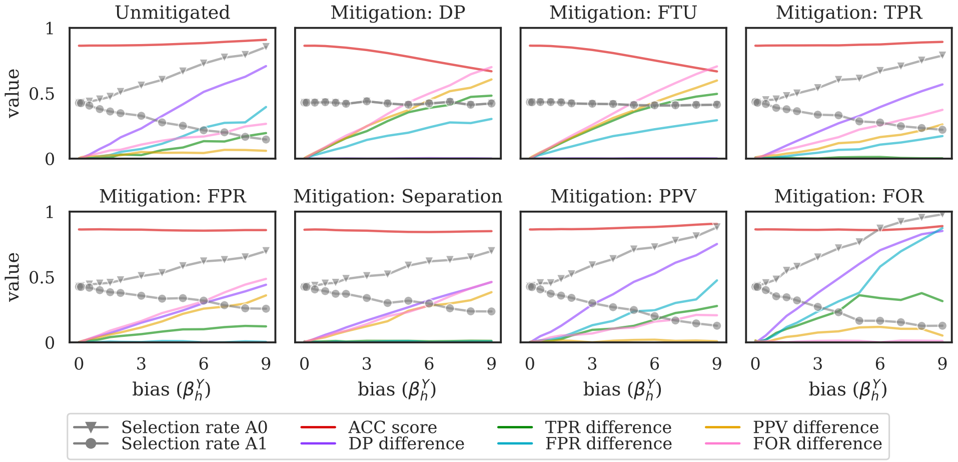


**(a) Historical bias on $Y$**

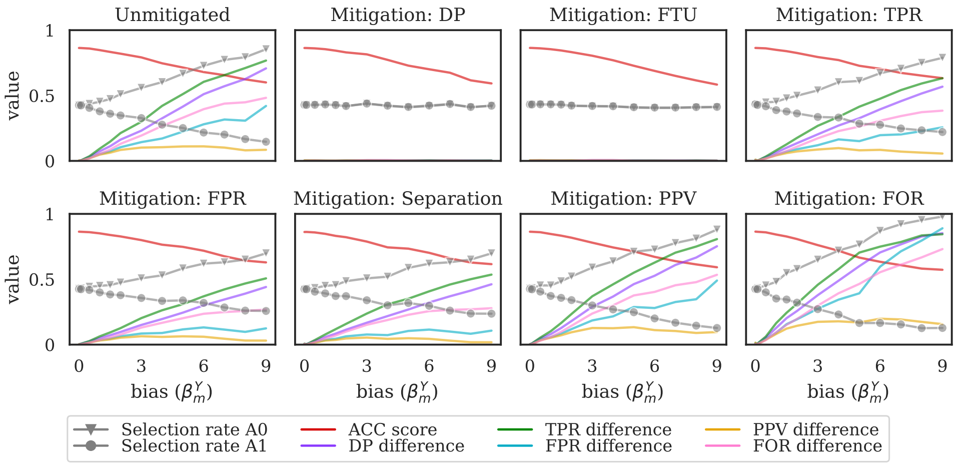


**(b) Measurement bias on $Y$**

**Figure S4: Accuracy and fairness metrics for biased labels $Y$ in the financial lending example (see section "Example 2: Biased Labels in Financial Lending" in the main paper). Notice that all metrics in (b) are computed with respect to the "true" target $Y$.**

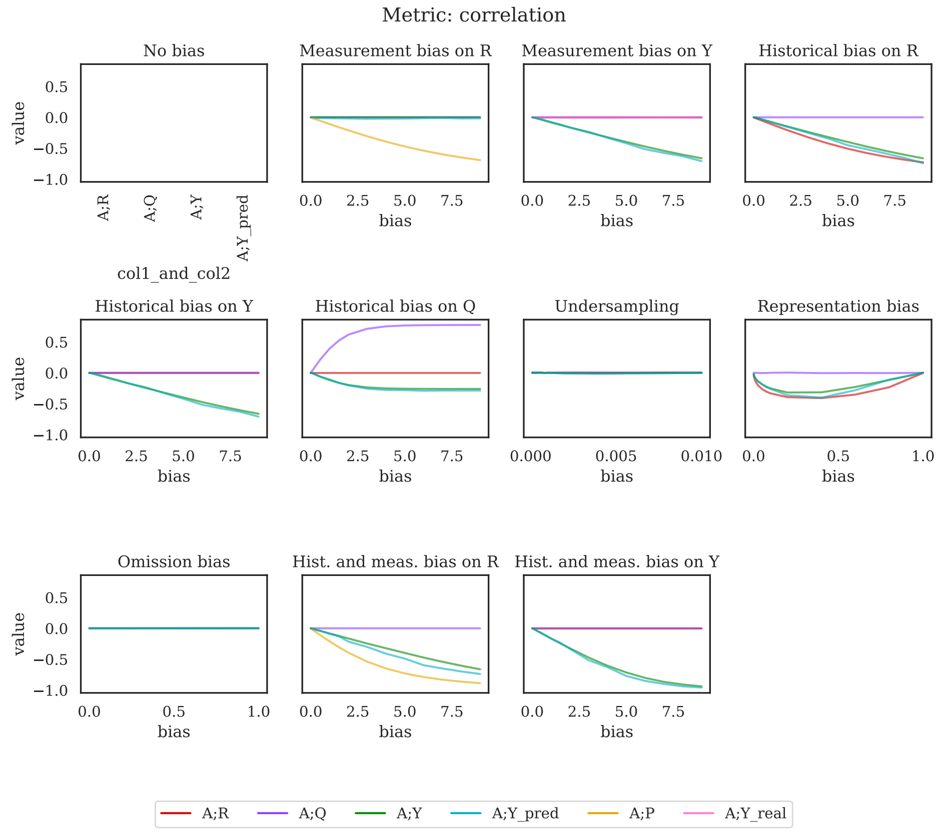


**Figure S5: Correlation between the sensitive attribute $A$ and the features, labels, and predictions. $Y$ denotes the observed label. In the case of measurement bias on $Y$, $Y_{real}$ stands for the the real unobserved $Y$.**

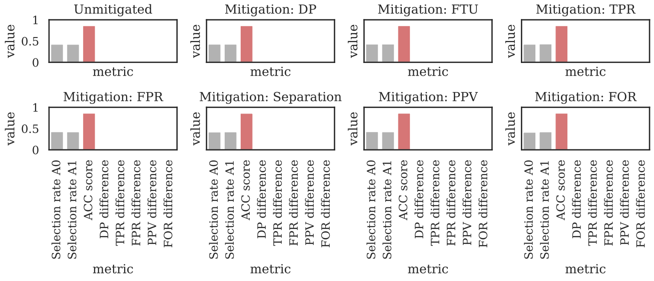


**(a) Accuracy and group fairness parity metrics**

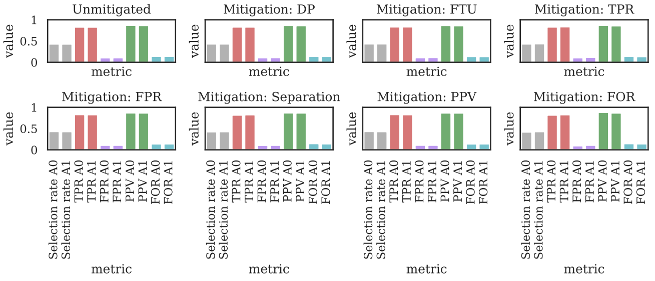


**(b) Group-specific fairness metrics**

**Figure S6: No bias**

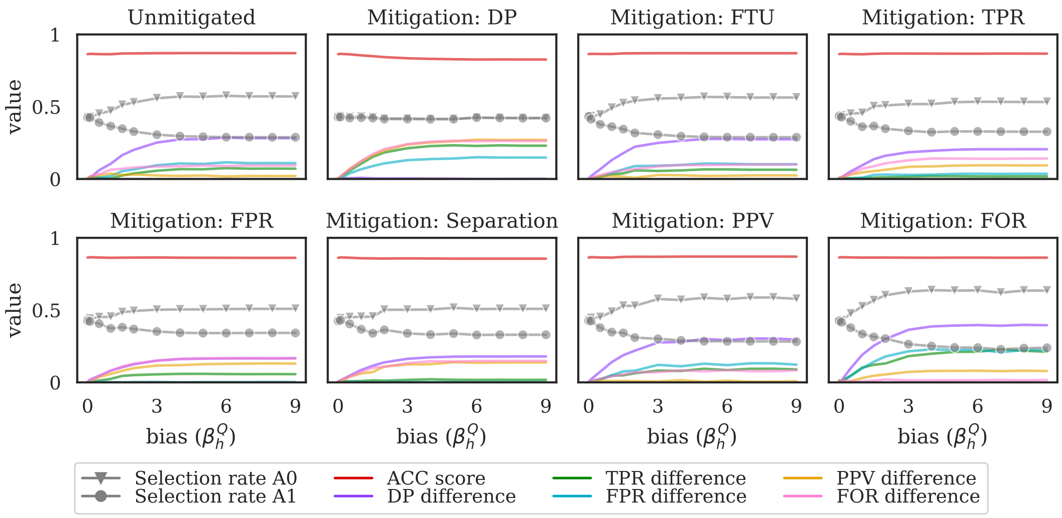


**Figure S7: Historical bias on $Q$**

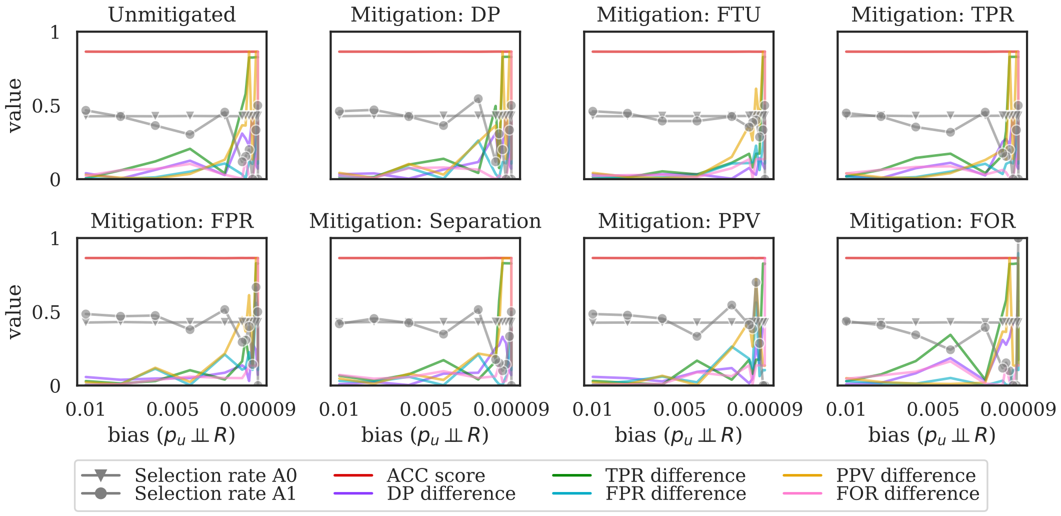


**Figure S8: Undersampling**

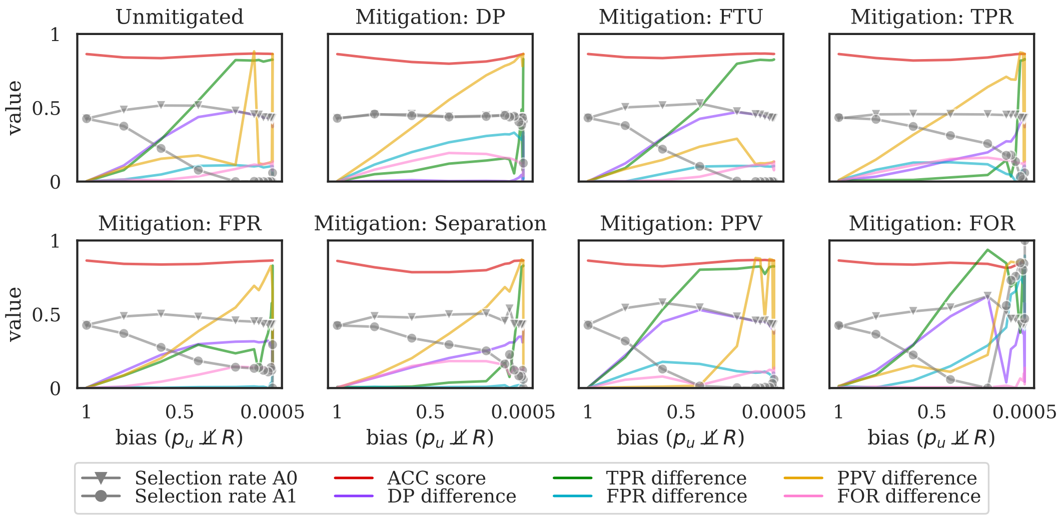


**Figure S9: Representation bias (undersampling conditional on $R$)**

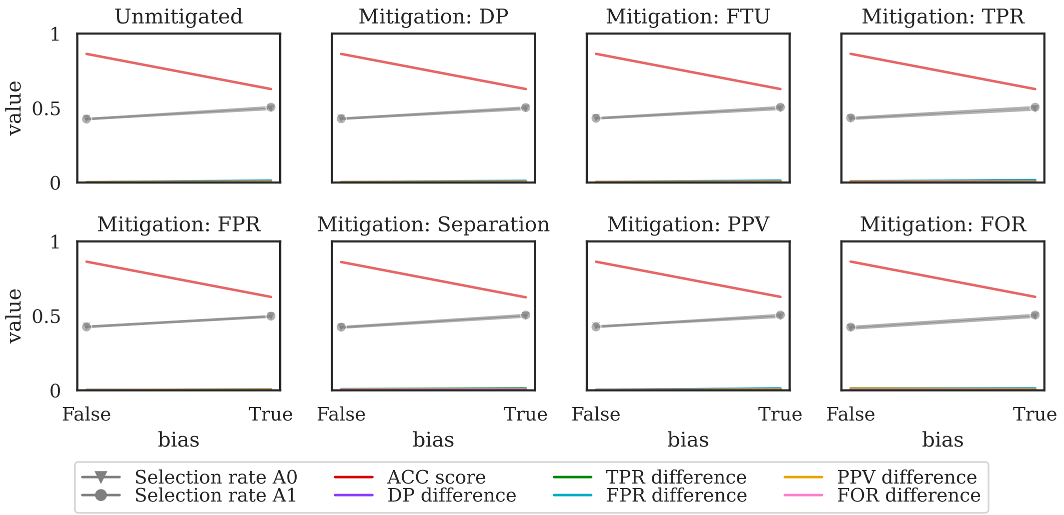


**Figure S10: Omission bias (omitting the feature $R$ – or its proxy $P_R$, in the case of measurement bias on $R$)**

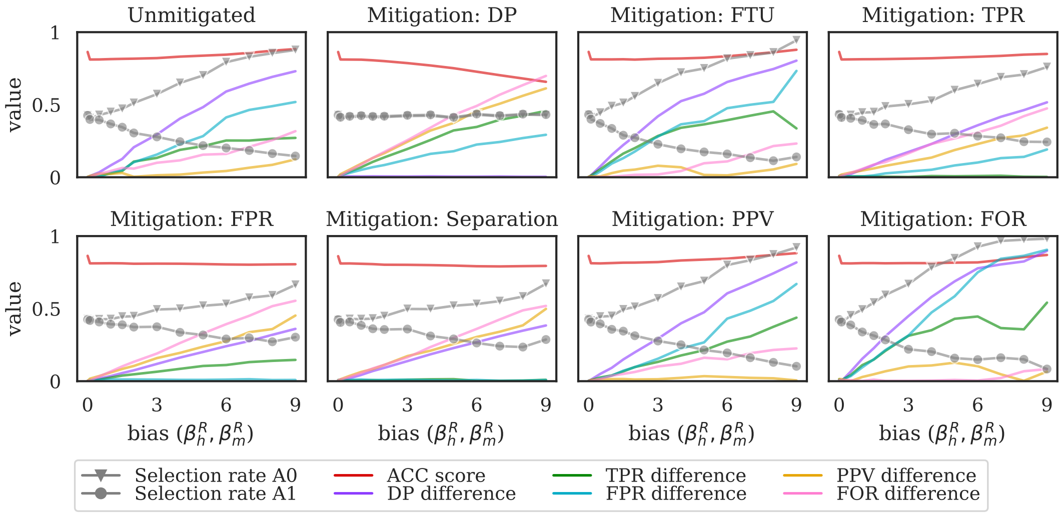


**Figure S11: Historical bias on $R$ and measurement bias on $R$**

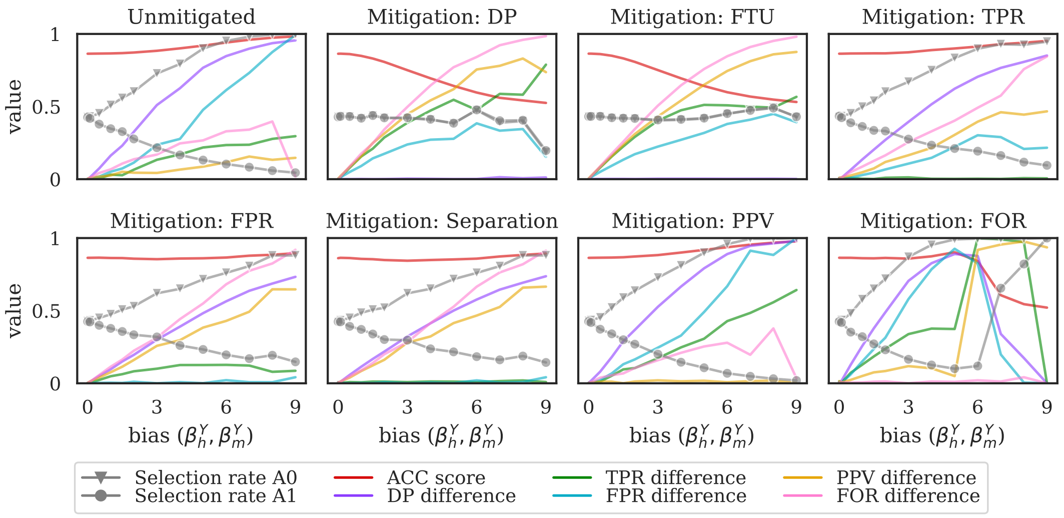


**Figure S12: Historical bias on $Y$ and measurement bias on $Y$**

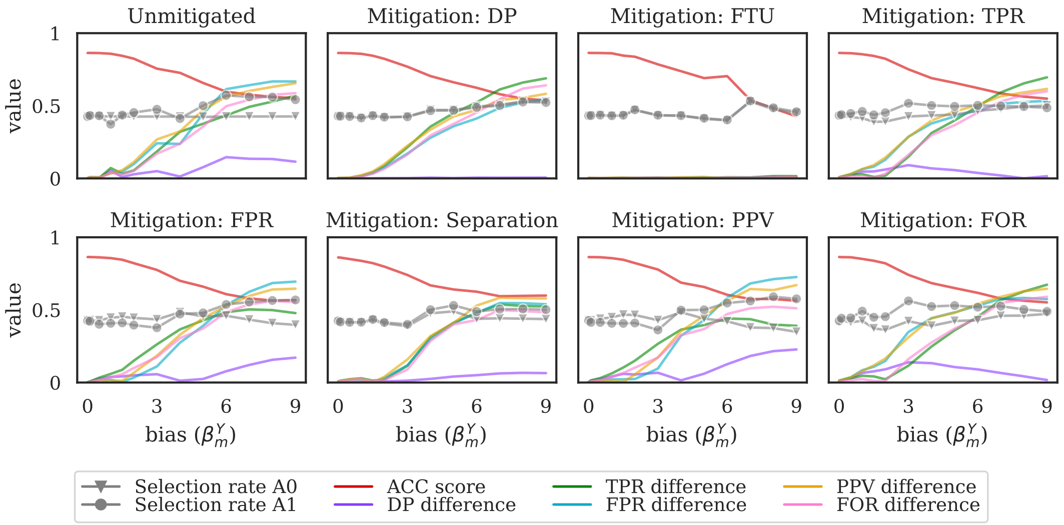


**Figure S13: Non-linear measurement bias on $Y$**
