# Supplementary material for: On the Societal Impact of Machine Learning
Source: arXiv:2510.23693 source file (2026-09-10)
Supplement: Supplementary file 2 [file paper6_Appendix.pdf]

## A UTILITY-WEIGHTED CONFUSION MATRIX

Table 1 shows a confusion matrix with the parameters ($u_{11}$, $u_{12}$, $u_{21}$, and $u_{22}$) used to weight the possible outcomes.

Table 1. Confusion matrix weighted with utilities

| | $Y = 1$ | $Y = 0$ |
|---|---|---|
| $D = 1$ | $u_{11}$ | $u_{12}$ |
| $D = 0$ | $u_{21}$ | $u_{22}$ |

## B PROOF OF LEMMA 2

Recall that the number of individuals assigned ($n_{D=1}$) can be written as $\sum_{i \in S} d_i$ and that the positive predictive value (PPV) is defined as:

$$PPV = P[Y = 1|D = 1] = \frac{1}{n_{D=1}} \sum_{i \in S} p_i d_i.$$

Suppose that $n_{D=1}$ is predefined and that the $PPV$ is given. For binary group membership $A$, the total utility $\tilde{U}$ can be written as:

$$\begin{aligned}
\tilde{U} &= \sum_{i \in S} \beta d_i + (\alpha - \beta) \sum_{i \in S} p_i d_i \\
&= \beta n_{D=1} + (\alpha - \beta)(PPV n_{D=1}) \\
&= \beta n_{D=1} + \alpha PPV n_{D=1} - \beta PPV n_{D=1} \\
&= (\alpha PPV + \beta(1 - PPV)) n_{D=1}.
\end{aligned}$$

Thus, for a given $PPV$ and a predefined selection capacity $n_{D=1}$, the total utility is given, and any decision rule that satisfies the constraint in Equation 5 is optimal.

## C OPTIMAL DECISION RULES UNDER FOR PARITY

In this section, we present the optimal solution for a utility-maximizing decision maker that wants to satisfy the group fairness metric false omission rate (FOR) parity. The FOR is defined as the average probability of individuals with $D = 0$ to have $Y = 1$, which can be written as $\frac{1}{n_{D=0}} \sum_{i \in S} p_i(1 - d_i)$, where $d_i$ is a binary multiplier representing the decision that is made for an individual $i$. The fairness definition FOR parity requires this value to be the same across groups. In the following, we interpret the decision problem as a *selection problem*, however, this time denoting individuals with $D = 0$ as "being selected."

Again, the solution is also composed of two consecutive steps. First, we derive the optimal decision rules $d^*$ for a simplified constraint: We assume that the FOR of both groups must be equal to a predefined value $FOR_t \in [0, 1]$. Then, we solve the full optimization problem by maximizing the decision maker's utility over all possible values of $FOR_t$.

We can translate this optimization problem into an equivalent problem, defining $\hat{u}_i$ as the *relative utility gain* when switching the decision from $D = 1$ to $D = 0$. So, $\hat{u}_i = 0$ for $D = 1$, and $\hat{u}_i = -\alpha p_i - \beta(1 - p_i)$ for $D = 0$. Thus, the

constrained optimization problem has the form:

$$\begin{aligned} \underset{d}{\arg\max} \quad & \hat{U} = \sum_{i \in S} \hat{u}_i (1 - d_i) \\ \text{subject to} \quad & \frac{1}{n_{A=a|D=0}} \sum_{j \in S_a} p_j (1 - d_j) = FOR_t, \quad \text{for } FOR_t \in [0, 1] \end{aligned} \tag{C.1}$$

where $S_a$ is the set of all individuals of group $a$, $n_{A=a|D=0}$ denotes the number of individuals in group $a$ with $D = 0$. Hence, the constraint describes a parity of the two groups' FORs. Since the FOR can only be defined if at least one individual is selected, we assume $n_{A=a|D=0} \geq 1$ for each group. The solution for the optimal decision rules while satisfying FOR parity across groups is analogous to the one under positive predictive value (PPV) parity (see Lemma 2 and Theorem 3 in the Section 3.4).

We first analyze case I with a simplified fairness constraint, where we assume that the FOR of both groups must be equal to a predefined value between 0 and 1, denoted by $FOR_t$. Suppose that $n_{D=1}$ is predefined, which is equivalent to $n_{D=0}$ being predefined. Similar to Lemma 2 (along with its proof in Appendix A), the total utility for an optimal solution satisfying FOR parity is:

$$\hat{U} = (-\alpha FOR_t - \beta(1 - FOR_t)) n_{D=0}. \tag{C.2}$$

Following similar reasoning as in the case of PPV parity, we end up with a conceptually identical solution for case I, where $n_{D=1}$ is predefined. Namely, for a given $FOR_t$, the total utility $\hat{U}$ is the same for any solution under FOR parity. Any decision rule $d(p, a)$ with $n_{D=1}$ that satisfies the constraint stated in Equation C.1 for a given $FOR_t$ is optimal. We thus end up with two independent selection problems, one for each group, which consists of finding a selection of individuals characterized by the fact that their average probability equals $FOR_t$. For each group $a$, selections with different numbers $n_{A=a|D=0}$ are possible. As long as the predefined $n_{D=0}$ is met, the group membership of the selected individuals does not matter for the resulting total utility. Hence, there may be several solutions to the optimization problem that differ regarding the number of individuals selected per group (i.e., representing different combinations of $(n_{A=0|D=0}, n_{A=1|D=0})$), with $n_{A=0|D=0} + n_{A=1|D=0} = n_{D=0}$. Note that most of these solutions violate the group fairness metric statistical parity while still meeting the fairness criterion of FOR parity.

We now analyze case II, where $n_{D=1}$ is not predefined. Equation C.2 directly shows that for values $FOR_t$ for which $-\alpha FOR_t - \beta(1 - FOR_t) < 0$, a decision maker who wants to maximize the total utility should minimize $n_{D=0}$, thus assigning the decision $D = 0$ only to one individual from each group, yielding a total utility of $\hat{U} = 2(-\alpha FOR_t - \beta(1 - FOR_t))$ for a binary protected attribute. In the following, we thus assume that $-\alpha FOR_t - \beta(1 - FOR_t) > 0$. Again we assume that the size of both groups is large but finite. Above we showed that, under these assumptions, the decision maker's goal is to find the selection that satisfies the constraint $FOR = FOR_t$ with the maximum $n_{D=0}$. Similarly to the solution for PPV parity (see Theorem 3), the total utility $\hat{U}$ is maximized with decision rules $d^*$ of the following form when applying FOR parity as a fairness constraint:

$$d_i^* = \begin{cases} \left.\begin{array}{ll} 0, & \text{for } p_i \geq \tau_a \\ 1, & \text{otherwise} \end{array}\right\} \text{for } FOR_t > BR_{A=a} \\ \left.\begin{array}{ll} 0, & \text{for } p_i \leq \tau_a \\ 1, & \text{otherwise} \end{array}\right\} \text{for } FOR_t < BR_{A=a}, \end{cases} \tag{C.3}$$

where $\tau_a$ denote different group-specific constants and $BR_{A=a}$ denotes group $a$'s base rate (BR) which is defined as the ratio of individuals belonging to the positive class ($Y = 1$): $BR_{A=a} = P[Y = 1|A = a] = \frac{1}{n_{A=a}} \sum_{i \in S_a} p_i$. The only

difference to the solution under PPV parity (see Equation 7) is the fact that decision rules of this form focus on the optimal selection of individuals with $D = 0$.

Finally, we perform the second step of the solution: from a discretization of all $FOR$, for which a solution exists, we choose the one that (in combination with the corresponding $n_{D=0}$) maximizes the total utility. Thereby, every $n_{D=0}$ is composed of the optimal selections $n_{A=a|D=0}$ for all groups $a \in A$, as elaborated in the first step of the solution.

## D ADDENDUM TO THE SYNTHETIC DATA EXAMPLE

Here we present additional results for the synthetic data example. Based on the three populations we introduced in Section 4.1, we show the resulting PPV and FOR for a utility-maximizing decision maker who want to satisfy PPV parity, FOR parity, or sufficiency.[1]

Figure 1 visualizes the three populations' solution spaces containing possible PPV-FOR combinations and the solutions that maximize utility – with or without the (relaxed) fairness constraints. Absent any fairness constraint, it is optimal for the bank to grant a loan to all individuals whose $p > t_0 = 0.3$. This is indicated with a group-specific cross (orange for group 0 and blue for group 1) in the Figures 1a-1c.

In populations 1 and 2, $PPV > max(BR_{A=a})$ and $FOR < min(BR_{A=a})$, thus, individuals with higher probability are preferred to those with lower probability. However, in population 3, the upper-bound threshold used for group 1 leads to $PPV_{t1,t2} < BR_{A=1}$ and $FOR_{t1,t2} > BR_{A=1}$ under PPV parity. The optimal combinations of $PPV$ and $FOR$ lie on $F_0(PPV_{A=0})$, representing optimal PPV-FOR combinations as introduced in Section 3.5, for group 0 (on $F_1(PPV_{A=1})$ for group 1), both for the solutions satisfying either PPV parity or FOR parity and for the solution without any fairness constraint. As we can clearly see in all three populations, one group needs to deviate from their optimal PPV-FOR combination to satisfy sufficiency, resulting in within-group unfairness. For all three populations in Figure 1, the advantaged group 1 is the one that deviates in order to maximize utility while satisfying sufficiency. However, this is not always the case as it depends on the utility function.[2]

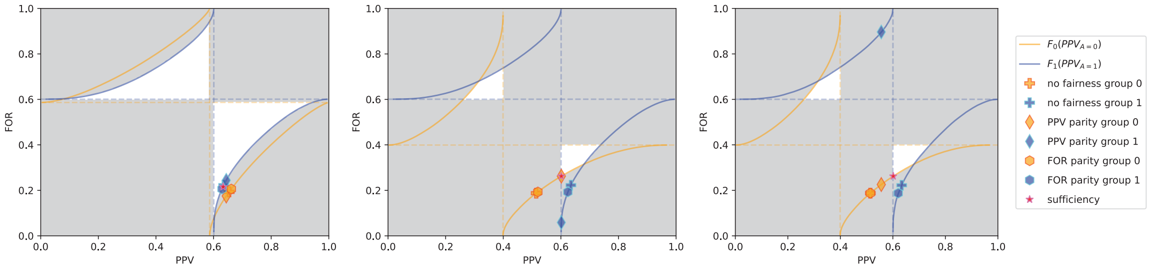


(a) Population 1 (b) Population 2 (c) Population 3

Fig. 1. Utility maximization under sufficiency or one of its relaxations for three different populations (synthetic)

[1]Data and code to reproduce our results are available at https://github.com/joebaumann/fair-prediction-based-decision-making.
[2]There are situations in which the disadvantaged group must deviate, as can be seen with those parts of the solution space that are bounded by $F_1(PPV)$.
