# Supplementary material for: On the Societal Impact of Machine Learning
Source: arXiv:2510.23693 source file (2026-09-10)
Supplement: Supplementary file 3 [file paper8_appendix.pdf]

# A Data Sources

Table 2 shows the data sources that were used for feature generation. Data from the court system on eviction was linked using a unique identifier to other county data, including demographics, enrollment in county/state programs, housing and homelessness services, and mental/behavioral health interactions. The dataset contains interactions between January 2012 and August 2023.

| Data Type | Info Entry Date | Information |
|---|---|---|
| **Demographics** | most recent interaction | ➢ gender, birthdate of individual, and (frequency of) address changes |
| **Evictions** | filing date<br>hearing date<br><br>OFP date | ➢ dollar amount claimed to be owed according to landlord<br>➢ who won the case (tenant or landlord)<br>➢ how much tenant owes landlord<br>➢ whether an OFP has been filed |
| **Program Interactions** | enrollment date<br><br>termination date | ➢ program type: i.e. Medicaid, Food Assistance, Homeless Shelter, Medical Assistance Transportation, or other similar programs offered by ACDHS<br>➢ when client is no longer enrolled in the program |
| **Public Housing** | enrollment date<br>move-in date<br>address change date | ➢ housing service type: i.e. Section 8 Voucher, Rapid Rehousing, or similar<br>➢ when and where client was rehoused (can be long after enrollment date)<br>➢ when and where client moves to a new location |
| **Mental & Behavioral Health** | interaction start date<br>interaction end date<br>diagnosis date | ➢ interaction type: i.e. walk-in, crisis, or hospital stay<br>➢ when person left (only relevant for multi-day stays)<br>➢ type of official diagnosis: i.e major depression, bipolar disorder, etc |
| **Physical Health (ER)** | interaction start date<br>interaction end date | ➢ when person visited the ER<br>➢ when person left (only relevant for multi-day stays) |
| **Children, Youth, and Families (CYF)** | interaction start date<br>interaction end date | ➢ interaction type: i.e. child moved to foster care or group home<br>➢ when the child moved to a different service or "aged out" (turned 18) |

Table 2: Sources of data used for feature generation, as well as the dates at which we consider each piece of information to be known for temporal validation.

**Mitigating Data Leakage.** Since we are using temporal validation, we need to ensure that, if we are evaluating an algorithm with data known up to a certain date, we do not use any information that was not known up to that date. Otherwise, we run the risk that the "leakage" of information from the future affects past results. For example, if we were to train a model on data up to January 1 2019 and a client had an eviction in December 2018 but an OFP in February, we must make sure we do not use any information about that individual's OFP in our training data. At first, this may not seem like a difficult task, but it can prove tricky with real-world, messy data. For each column given to us by ACDHS, when did they know that data by? Do they update that data daily, weekly, or even monthly? Considering these questions is crucial to ensure that our models do not appear to perform better than they would when actually deployed, in case we were inadvertently using information only known in the future. For this reason, we not only explain the type of information provided by ACDHS in Table 2, but also specify which date we know that information by.

As shown in Table 2, most data is associated with a specific interaction, allowing us to generate a temporal history for each client. However, this is not the case for demographic information, as this is continuously updated without keeping track of old

entries. Consequently, the dataset only reveals what demographic information was known about an individual at the time of the most recent interaction. Certain demographic information, such as race, are more likely to be `null` for individuals with few interactions with ACDHS. Using this information is problematic for temporal validation since it contains important information from the future (i.e., whether an individual had many interactions with ACDHS up to the last day in the dataset. This, in turn, could falsify the performance evaluation results as individuals falling into homelessness interact more with ACDHS, on average. To avoid this type of data leakage, we made sure to only use demographic information that is collected during every interaction.

# B Demographic Composition of Cohort

Table 3 describes the demographic composition of the last pre-pandemic cohort as of January 1, 2019. In this cohort (as in others), Women and African Americans are disproportionately at risk of facing eviction, and, conditional on facing eviction, are at higher risk of future homelessness. Fourteen percent of the population in Allegheny County is African American (U.S. Census Bureau 2022), yet this share jumps to 55% among those facing eviction and to 59% among those facing eviction that fall into homelessness the following year. Those with a history of homelessness are also more likely to reenter homelessness in the future: while 6% of individuals in the cohort had been homeless in the past, this share jumps to 37% among those who end up in homelessness in the following year.

| **Characteristics** | **Total** | **Becomes homeless** | |
|---|---|---|---|
| | | *No* | *Yes* |
| Female | 56.5% | 56.4% | 61.4% |
| African American | 55.1% | 55.0% | 58.6% |
| Has been homeless | 6.0% | 5.4% | 37.1% |
| | *(N=4036)* | *(N=3966)* | *(N=70)* |

Table 3: Demographic composition of cohort as of January 1, 2019 across key demographic groups of interest and label outcomes.

# C Parameter Grid

Table 4 shows the different parameter values that were used for the models. Models with each possible combination of these hyperparameters were trained and tested for each date of analysis.

# D Temporal Validation

Figure 5 visualizes the temporal validation splits. The results of splits 1 – 18 are reported inSection 5. The results of the shadow mode deployment are reported in Section 6.1.

For each temporal split, we generate feature label pairs that span the entire timespan of the training set. As an example, we visualize this for the split 10 in Figure 6. The split 10 of the temporal validation corresponds to the model development as of January 1 2019. Thus, the most recent label timespan considered in the training data matrix is between January 1 2018 and January 1 2019. However, individuals who only made use of homelessness services before January 1 2018 are not labeled positively in this label timespan. Therefore, we additionally consider label timespans of 12 months, going back in 3 months intervals until January 1 2013. This is needed to exploit the data available in the training set while respecting the temporal flow of events in the past.

# E Additional Baselines

In addition to the baselines mentioned in Section 4.4, we also tried a few others. These were omitted from the paper due to their poor performance.

B4. **Age at first interaction.** This baseline sorts by the age at which the individual first was enrolled in an ACDHS program. The younger the individual at their first interaction, the more likely they are to fall into homelessness.

B5. **Age at first adult interaction.** Some individuals are involved in child welfare or foster care services from a young age. This baseline extends B4 by only considering ACDHS program involvement once the individual is an adult (18 years of age).

B6. **Days since current filing.** Similar to *B1: Current process*, this baseline instead sorts individuals by the date of their current eviction filing (not their OFP date), with earlier dates being considered as more likely to fall into homelessness.

B7. **Days since last program involvement.** This baseline assumes that individuals who recently interacted with non-homelessness ACDHS services are more vulnerable, and therefore more likely to fall into homelessness.

B8. **Number of distinct programs.** This baseline sorts individuals by the number of distinct ACDHS programs they have been involved in throughout their lifetime, with more programs indicating that the individual is more vulnerable and therefore more likely to fall into homelessness.

| Model Name | Parameter | Values |
|---|---|---|
| **Logistic Regression** | *C* | `0.001, 0.01, 0.1, 1` |
| | *Penalty* | `L1, L2` |
| **Decision Tree** | *Max depth* | `1, 2, 5, 10, no limit` |
| | *Min samples split* | `2, 10` |
| **Random Forest** | *Number of estimators* | `1000, 5000, 10000` |
| | *Max depth* | `5, 10, 25, 50` |
| | *Min samples split* | `10, 100` |
| | *Min samples leaf* | `10, 100` |
| **Light GBM** | *Boosting type* | `dart` |
| | *Number of estimators* | `100, 300, 500` |
| | *# leaves* | `31` |
| | *Max depth* | `10, 100` |
| **XG Boost** | *Booster* | `gbtree` |
| | *Learning rate* | `0.01, 0.1` |
| | *Number of estimators* | `100, 300` |
| | *Max depth* | `5, 10, 40` |

Table 4: Grid search parameters for model selection

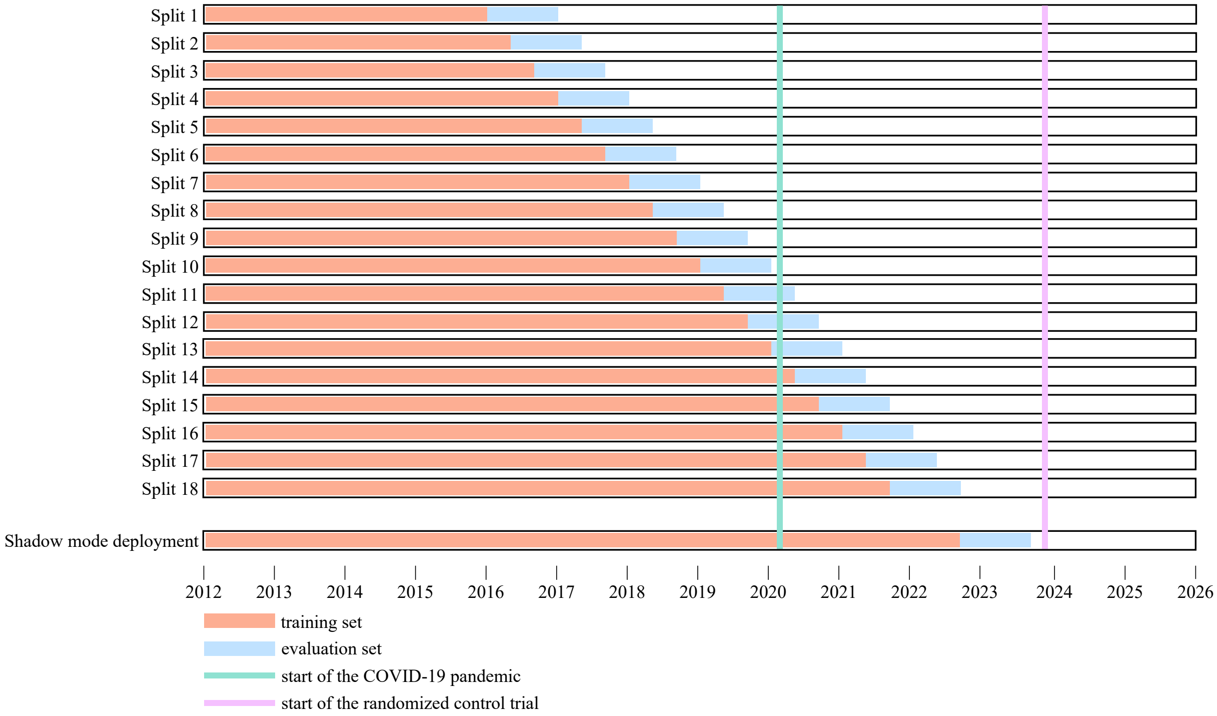


Figure 5: Temporal validation

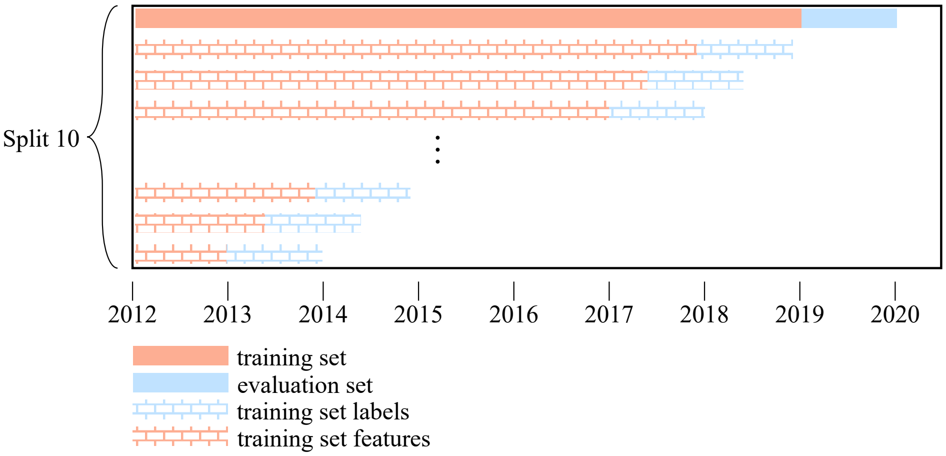


Figure 6: Feature label pair generation in one temporal validation split (here we represent split 10 as an example)

B9. **Number of program involvement spells.** Since an individual can be enrolled in the same ACDHS program multiple times throughout their lifetime, this baseline extends B9 by considering the distinct number of times an individual has been involved in any ACDHS program, with more involvement indicating the individual is more likely to fall into homelessness.

B10. **Total days in program involvement.** Similar to the previous two baselines, this baseline sorts individuals by the total number of days they have been involved in any ACDHS service, with more involvement indicating the individual is more likely to fall into homelessness.

Figure 7 shows how these baselines perform compared to our selected baselines B1 — B3. We see that generally, *B2: Previous Homelessness* performs better than other baselines. Though *B1: Current Process* and *B3: Baserate* also do not perform well, they were included in the main results as B1 most closely emulates ACDHS' current process and B3 shows how well random allocation would perform.

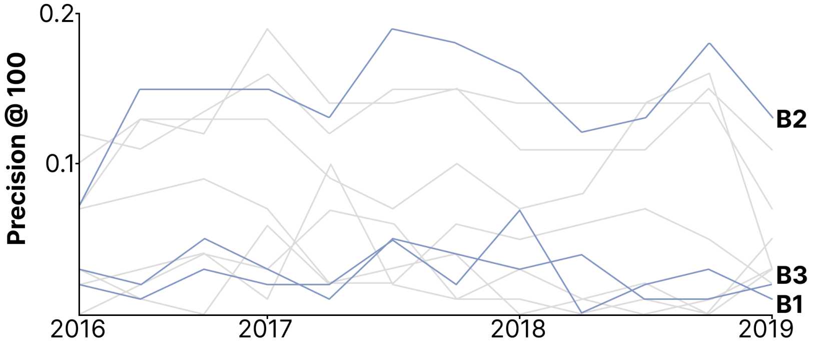


Figure 7: Performance of all attempted baselines: the grey lines showcase the performance of B4 — B10 which were omitted from the main paper results since they all perform less well than *B2: Previous Homelessness*.

## F Effect of the COVID-19 pandemic on cohort size and positive label prevalence

Figure 8a shows that, due to the eviction moratorium, the number of cases drops drastically in the year 2020. However, after the moratorium, the number of eviction cases rises almost to pre COVID-19 pandemic level in the year 2022. As can be seen in Figure 8b, the cohort size also changes accordingly in this time period – as does the number of positive labels in those cohorts, see Figure 8c.

## G Field Trial Schematic Design

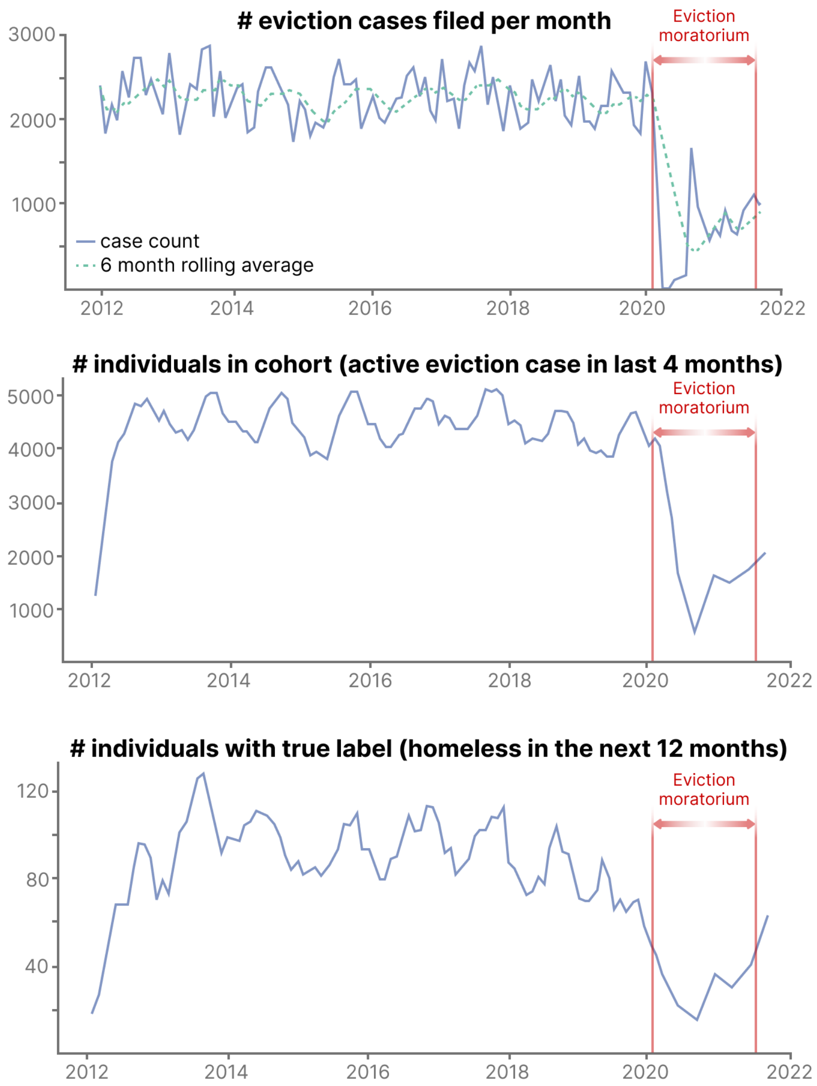


Figure 8: (a) Number of eviction cases filed per month, (b) number of individuals in the cohort as of a particular date of analysis, and (c) number of individuals with that become homeless in the next 12 months as of a date of analysis.

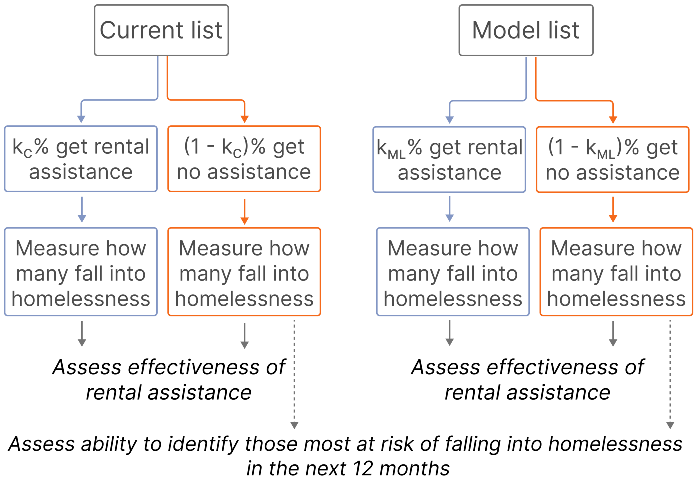


Figure 9: Schematic drawing of RCT design
